# Supplementary material for: Optimal nonlinear coherent mode transitions in Bose-Einstein Condensates utilizing spatio-temporal controls
Source: arXiv:1603.08475 source file (2016-03-28)
Supplement: Supplementary file 1 [file hocker_supp.pdf]

# Optimal nonlinear coherent mode transitions in Bose-Einstein Condensates utilizing spatio-temporal controls: Supplementary Material

## I. VARIATIONAL CONTROL EQUATIONS FOR THE GPE

A canonical method for obtaining the sufficient conditions for optimal controls is through adapting a cost functional to guide the underlying system dynamics while assuring that the GPE is satisfied by an enforcing Lagrange multiplier [**?** ]. Using this method, the variational control relations in eqs. (8)-(12) for optimal state-to-state transitions with the GPE are derived here. Introducing the functional Lagrange multiplier function $p(x,t)$, a constraint can be added to eq. (2) such that dynamics of the GPE in eq. (4) are followed, along with its complex conjugate. This modified cost functional $\tilde{J}$, is given as

$$\begin{aligned}
&\tilde{J}[\psi,\psi^*,p,p^*,V,g] \\
&= \left| \int \phi_f^*(x)\psi(x,T)dx \right|^2 + \\
&\int_0^T \int_{-\infty}^{\infty} p^*(x,t)\left(-i\hbar\dot{\psi}(x,t) + H[\psi,\psi^*,V_{\text{cont}},g_{\text{cont}}](x,t)\psi(x,t)\right) + \\
&\left(i\hbar\dot{\psi}^*(x,t) + \psi^*(x,t)H[\psi,\psi^*,V_{\text{cont}},g_{\text{cont}}](x,t)\right)p(x,t)dxdt \qquad \text{(S1)}
\end{aligned}$$

where this equation is an explicit expansion of $\text{Re}(\cdot)$ in eq. (7). The overhead dot denotes $\partial/\partial t$, and the Hamiltonian $H[\psi,\psi^*,V_{\text{cont}},g_{\text{cont}}]$ is shown here to explicitly depend upon the wavefunction, its complex conjugate, as well as the controls $V_{\text{cont}}$ and $g_{\text{cont}}$. Introducing the Lagrange multipliers $p$ and $p^*$ lifts the implicit constraint that $\psi$, and $\psi^*$ are dependent upon the controls, so functional variations of $J$ can now be independently considered. Setting $\delta J/\delta\psi(x,t)$ and $\delta J/\delta p(x,t)$, as well as their complex conjugates equal to zero, in addition to determining $\delta J/\delta V_{\text{cont}}(x,t)$ and $\delta J_{\text{cont}}/\delta g(x,t)$, gives the variational equations that optimize $J$. $V_{\text{cont}}$ and $g_{\text{cont}}$ are strictly real to assure that the Hamiltonian is Hermitian.

The first derivatives $\delta\tilde{J}/\delta p(x,t)$ and $\delta\tilde{J}/\delta p^*(x,t)$ are

$$\frac{\delta\tilde{J}}{\delta p(x,t)} = i\hbar\dot{\psi}^*(x,t) + \psi^*(x,t)H[\psi,\psi^*,V_{\text{cont}},g_{\text{cont}}](x,t) \qquad \text{(S2)}$$

$$\frac{\delta\tilde{J}}{\delta p^*(x,t)} = -i\hbar\dot{\psi}(x,t) + H[\psi,\psi^*,V_{\text{cont}},g_{\text{cont}}](x,t)\psi(x,t). \qquad \text{(S3)}$$

Setting these two equations equal to zero yields the time-dependent GPE, and its complex conjugate equation,

$$i\hbar\dot{\psi}(x,t) = H[\psi,\psi^*,V_{\text{cont}},g_{\text{cont}}](x,t)\psi(x,t) \qquad \text{(S4)}$$

$$-i\hbar\dot{\psi}^*(x,t) = \psi^*(x,t)H[\psi,\psi^*,V_{\text{cont}},g_{\text{cont}}](x,t) \qquad \text{(S5)}$$

Next, the variations with respect to the controls are

$$\begin{aligned}
\frac{\delta\tilde{J}}{\delta V_{\text{cont}}(x,t)} =& p^*(x,t)\frac{\partial H[\psi,\psi^*,V_{\text{cont}},g_{\text{cont}}](x,t)}{\partial V_{\text{cont}}(x,t)(x,t)}\psi(x,t) + \\
&\psi^*(x,t)\frac{\partial H[\psi,\psi^*,V_{\text{cont}}(x,t),g_{\text{cont}}(x,t)](x,t)}{\partial V_{\text{cont}}(x,t)}p(x,t) \\
&= p^*(x,t)\psi(x,t) + \psi^*(x,t)p(x,t) \\
&= 2Re\left[p^*(x,t)\psi(x,t)\right], \qquad \text{(S6)}
\end{aligned}$$

and

$$\begin{aligned}\frac{\delta \tilde{J}}{\delta g_{\text{cont}}(x,t)} =& p^*(x,t)\frac{\partial H[\psi,\psi^*,V_{\text{cont}},g_{\text{cont}}](x,t)}{\partial g_{\text{cont}}(x,t)(x,t)}\psi(x,t)+ \\ & \psi^*(x,t)\frac{\partial H[\psi,\psi^*,V_{\text{cont}},g_{\text{cont}}](x,t)}{\partial g_{\text{cont}}(x,t)}p(x,t) \\ &= p^*(x,t)|\psi(x,t)|^2\psi(x,t)+\psi^*(x,t)|\psi(x,t)|^2 p(x,t) \\ &= 2Re\left[p^*(x,t)|\psi(x,t)|^2\psi(x,t)\right].\end{aligned} \tag{S7}$$

Finally, the equations for $p$ and $p^*$ must be calculated from determination of $\delta\tilde{J}/\delta\psi(x,t)$ and $\delta\tilde{J}/\delta\psi^*(x,t)$. First $\delta\tilde{J}/\delta\psi(x,t)$ is expressed as

$$\begin{aligned}\frac{\delta \tilde{J}}{\delta \psi(x,t)} =& \\ & \delta(t-T)\delta(x'-x)\left[\phi_f^*(x')\left(\int_{-\infty}^{\infty}\phi_f(x')\psi^*(x',t)dx'\right)+-i\hbar p^*(x,t)\right] \\ & + i\hbar\dot{p}^*(x,t)+p^*(x,t)H[\psi,\psi^*,V_{\text{cont}},g_{\text{cont}}](x,t) \\ & p^*(x,t)\frac{\partial H[\psi,\psi^*,V_{\text{cont}},g_{\text{cont}}](x,t)}{\partial\psi(x,t)}\psi(x,t)+ \\ & + \psi^*(x,t)\frac{\partial H[\psi,\psi^*,V_{\text{cont}}(x,t),g_{\text{cont}}(x,t)](x,t)}{\partial\psi(x,t)}p(x,t),\end{aligned} \tag{S8}$$

where integration by parts was utilized to obtain the $\psi(x,t)$ and $\dot{p}(x,t)$ terms. Setting this derivative equal to zero yields the equation for $p^*(x,t)$,

$$\begin{aligned}-i\hbar\dot{p}^*(x,t) =& p^*(x,t)\left[H[\psi,\psi^*,V_{\text{cont}},g_{\text{cont}}](x,t)+g(x,t)|\psi(x,t)|^2\right] \\ & + g(x,t)\psi^{*2}(x,t)p(x,t) \\ & + \delta(t-T)\delta(x'-x)\left[\phi_f^*(x')\left(\int_{-\infty}^{\infty}\phi_f(x')\psi^*(x',t)dx'\right)-i\hbar p^*(x,t)\right].\end{aligned} \tag{S9}$$

Following a similar procedure for the calculation of $\delta\tilde{J}/\delta\psi^*(x,t)$ and setting it equal to zero yields

$$\begin{aligned}i\hbar\dot{p}(x,t) =& \left[H[\psi,\psi^*,V_{\text{cont}},g_{\text{cont}}](x,t)+g(x,t)|\psi|^2\right]p(x,t) \\ & + g(x,t)p^*(x,t)\psi^2(x,t) \\ & + \delta(t-T)\delta(x'-x)\left[\phi_f(x')\left(\int_{-\infty}^{\infty}\phi_f^*(x')\psi(x',t)dx'\right)+i\hbar p(x,t)\right].\end{aligned} \tag{S10}$$

Equations (**??**) and (**??**) can be separated into dynamical equations for $p$ and initial conditions, assuming that $p$ is a continuous function. To demonstrate this, consider integrating both sides of eq. (**??**) in a small window of time $\Delta\tau$ and space $\Delta x$ about $T$ and $x$, respectively,

$$\begin{aligned}&\int_{T-\Delta\tau}^{T+\Delta\tau}\int_{x-\Delta x}^{x+\Delta x} i\hbar\dot{p}(x'',t'')dx''dt'' = \int_{T-\Delta}^{T+\Delta}\int_{x-\Delta x}^{x+\Delta x}\left(H[\psi,\psi^*,V_{\text{cont}},g_{\text{cont}}](x'',t'')p(x'',t'')+\right. \\ & g(x'',t'')|\psi(x'',t'')|^2 p(x'',t'')+g(x'',t'')p^*(x'',t'')\psi^2(x'',t'')+ \\ & \left.\delta(t''-T)\delta(x''-x)\left[\phi_f(x'')\left(\int_{-\infty}^{\infty}\phi_f^*(x')\psi(x',t')dx'\right)+i\hbar p(x'',t'')\right]\right)dx''dt''.\end{aligned} \tag{S11}$$

Taking the limit of $\Delta\tau$ and $\Delta x$ going to zero, the left side of eq. (**??**) will go to zero by continuity of $p$,

as will the first 3 terms on the right hand side of the equation. The delta functions in $t''$ and $x''$, though, produce the final time condition in this limit:

$$p(x,T) = -\frac{i}{\hbar}\phi_f(x)\left(\int_{-\infty}^{\infty}\phi_f^*(x')\psi(x',T)dx'\right) \tag{S12}$$

In summary, the control equations for the one dimensional GPE are given below:

$$i\hbar\dot{\psi}(x,t) = H(x,t)\psi(x,t), \quad \psi(x,0) = \phi_0(x) \tag{S13}$$

$$-i\hbar\dot{\psi}^*(x,t) = \psi^*(x,t)H(x,t) \quad \psi^*(x,0) = \phi_0^*(x) \tag{S14}$$

$$\frac{\delta\tilde{J}}{\delta V_{\text{cont}}(x,t)} = Re\left[p^*(x,t)\psi(x,t)\right] \tag{S15}$$

$$\frac{\delta\tilde{J}}{\delta g_{\text{cont}}(x,t)} = Re\left[p^*(x,t)|\psi(x,t)|^2\psi(x,t)\right] \tag{S16}$$

$$-i\hbar\dot{p}^*(x,t) = p^*(x,t)\left[H^*(x,t) + g(x,t)|\psi(x,t)|^2\right] + g(x,t)\psi^{*2}(x,t)p(x,t), \tag{S17}$$

$$p(x,T) = -\frac{i}{\hbar}\phi_f(x)\left(\int_{-\infty}^{\infty}\phi_f^*(x')\psi(x',T)dx'\right) \tag{S18}$$

$$i\hbar\dot{p}(x,t) = \left[H(x,t) + g(x,t)|\psi|^2\right]p(x,t) + g(x,t)p^*(x,t)\psi^2(x,t), \tag{S19}$$

$$p^*(x,T) = \frac{i}{\hbar}\phi_f^*(x)\left(\int_{-\infty}^{\infty}\phi_f(x')\psi^*(x',T)dx'\right) \tag{S20}$$
